# Supplementary material for: Modeling Distinct Human Interaction in Web Agents
Source: arXiv:2602.17588 source file (2026-07-07)
Supplement: Supplementary file 1 [file discussions.tex]

\section{Discussions}

\subsection{Summary of Findings}

Our study explored how users collaborate with AI agents to accomplish web-based tasks.
% in both standardized and self-directed settings. 
Rather than acting merely as supervisors or correctors, users took on the role of active collaborators—adapting their behavior, offering guidance, and at times relying on the agent to explore or execute subtasks independently.

One consistent theme was trust through shared control. Although the agent led most interactions, users felt comfortable knowing they could step in when needed. This duality, where agents handle routine navigation while humans maintain strategic oversight, seemed to offer reassurance. This sense of agency was not rooted in the frequency of input but in the ability to shape outcomes when necessary.

Another emergent pattern was how task framing and ownership affected collaboration. In the free-form setting, where participants defined their own tasks, users were more inclined to let the agent operate independently. We can describe this process as \textit{delegating} rather than \textit{co-navigating} — i.e. how the framing of a task shifted the task outcome. In contrast, standard tasks, where goals (i.e., task descriptions) were defined \textit{a priori}, encouraged more frequent interventions and closer monitoring.

We also observed how users adapted their strategies in real-time. Many of them developed routines for pausing the agent before error-prone UI elements, waiting for completion before suggesting corrections, or stepping in only when progress stalled. These behavioral patterns reflect a developing mental model—a growing understanding of when, why, and how to intervene. 
% The agent was not treated as infallible, but as a capable partner whose gaps were both predictable and manageable.

\subsection{Unlocking Collaboration Through Intervention}
% -- agentic aversion
Intervention is not a workaround for failure --- rather, a central mechanism that makes a task successful. In our study, when users stepped in, it was not just to fix errors. They were clarifying ambiguity, expressing intent, and reasserting agency in tasks. These interventions made the agent more usable, not less.

Rather than striving for full automation, our findings support a more interactive vision: \textbf{agents that expect and embrace human guidance}. This echoes recent concerns about building fully autonomous systems for everyday use, which argue that such systems cannot adequately account for the complexity of human goals and environments \cite{fullno}. Our findings further demonstrate that real-world collaboration demands more than autonomy—it demands adaptability and shared control.

The ability of intervention also served as a powerful tool against algorithm aversion \cite{dietvorst2015algorithm}. Instead of disengaging after mistakes, participants had the opportunity to adjust the agent’s behavior and continue the task. Because they could intervene, users retained trust --- even when the agent misfired. They did not expect perfection; they expected the ability to course-correct.

These interactions often took on a collaborative tone: users spoke of ``helping the agent out'' or ``steering it back'', revealing a subtle but meaningful shift in the collaboration dynamics. Intervention became a way to build trust, maintain momentum, and co-own outcomes. 

\textbf{Even beyond real-time collaboration, we can utilize {\sc CowCorpus} with RLHF} (Reinforcement Learning from Human Feedback) \cite{bai2022training} to build better agents that are aligned with human preferences. Incorporating these patterns can enable agents to mimic user preferences and learn how to recover from dead ends.

\subsection{Considerations for Evaluating Agents in Real-World Contexts}

% -- how we mitigated concerns about safety
% -- how to design tasks and be aware of the LLM randonmess or hallucination
% -- why picking fixed vs free is good
% -- consideration for user privacy: give them options to share the data if they want rather than implicitly requesting them to do so.
% -- time consideration
% -- large trajectory, storage consideration

Evaluating collaborative agents in real-world contexts presents unique methodological challenges and design opportunities. Our study highlights several key considerations for setting up such evaluations.

\paragraph{Task Diversity Matters} 
A mix of fixed benchmark tasks and open-ended, user-defined tasks is helpful in capturing a bigger spectrum of agent capabilities. While benchmark tasks provide standardization for comparative analysis, free-form tasks better reflect the idiosyncratic nature of everyday web use. The contrast between the two also reveals how users naturally adapt their prompting strategies, and where agents are most likely to fail due to ambiguity \cite{zamfirescu2023johnny}.

%\paragraph{Human Feedback Should Be Native, Not Scripted} 
% We opted for self-initiated intervention logging and post-task annotations rather than rigid observation or artificial interruption prompts. This approach respects the user's natural workflow and captures more authentic moments of friction. Our results suggest that many interventions are subtle and strategic—not just reactive to error—which would be missed in scripted setups.

\paragraph{Human Feedback Should Be Organic, Not Scripted} 
Participants were given full control over when to pause, resume, or override the agent, which proved essential not just for safety, but also for confidence and exploration. Any real-world evaluation setup should prioritize transparency and freedom to encourage participants to experiment and engage freely with the agent.

\paragraph{Privacy and Consent Cannot Be Assumed}
We emphasized that participants can voluntarily opt in or opt out of sharing their data logs. Rather than having a server-based data annotation paradigm, we purposefully gave them the freedom to download the data log \textit{after} the task is completed. This paradigm ensures that users are fully in control and make a well-informed decision after observing the task outcome. Researchers should provide options to ensure users know what is being collected and why, especially when tasks involve personal workflows.

Finally, \textit{randomness in LLM behavior} --- an issue in both agent output and task outcomes --- adds noise to the annotated data \cite{rawles2024androidworld}. Researchers need to be mindful of such concerns and look for ways to mitigate such randomness as much as possible.

% \subsection{Limitation and Future Work}
% Currently, \cc annotation uses only \texttt{GPT-4o} as its LLM backbone. So, the results might be limited to the current reasoning capacity of \texttt{GPT-4o}. In the future, we would like to explore how we can use \cc to build a \textit{personalized AI agent} for each participant, aware of their individual preference and task description style.

% The study contributes to ongoing conversations around the limits of autonomy in interactive systems. As others have argued, fully autonomous agents are often misaligned with real-world complexity and user needs. Our findings reinforce this view, highlighting the importance of keeping humans in the loop—not simply to supervise, but to shape, direct, and recover the interaction as it unfolds.

% In supporting this kind of collaboration, intervention becomes more than an error-handling mechanism; it becomes a \textcolor{red}{design principle}. One that allows systems to work alongside people—not apart from them.
